# Supplementary material for: Lorentz group equivariant autoencoders
Source: arXiv:2212.07347 source file (2023-06-10)
Supplement: Supplementary file 1 [file appendix-recons.tex]

\subsection{Reconstruction}
\label{app:recons}
\subsubsection*{Cartesian Coordinates}
Since the input of the LGAEs is $(E, p_x, p_y, p_z)$, we also computed the reconstruction relative errors in the original coordinates, as shown in \cref{tab:lgae-rel-err-cartesian}. As expected, in terms of the four metrics, the LGAEs reconstruct what they were trained to learn better than particle $(p_\mathrm{T}^\mathrm{rel}, \eta^\mathrm{rel}, \phi^\mathrm{rel})$.
% In addition, \cref{tab:lgae-jet-rel-err-polar} shows the statistical information of relative errors of the reconstructed jet momenta in lab polar coordinates.

\begin{table*}[ht]
    \centering
    \caption{Median, IQR, IDR, and MAD of relative errors in particle feature
        $(p_x, p_y, p_z)$ reconstructions
        by LGAE models with min-max and mean aggregations and different latent 4-vector multiplicities ($\tau_{(1/2, 1/2}))$}
    \label{tab:lgae-rel-err-cartesian}
    \begin{tabular}{c|c|c|c|c|c}  \toprule
        Aggregation & $\tau_{(1/2,1/2)}$ & Median            & IQR               & IDR               & MAD               \\ \hline
        \multirow{2}{*}{min-max}
        % & $1$ ($16.7\%$) & $0.0342$ & $0.8414$ & $3.6891$ & $0.5273$ \\
        % & $2$ ($30\%$) & $-0.1810$ & $0.4783$ & $1.7325$ & $0.3525$ \\
        % & $3$ ($43.3\%$) & $0.0751$ & $0.6908$ & $2.7527$ & $0.4059$ \\
                    & $4$ ($56.7\%$)     & $-0.0892$         & $\mathbf{0.4128}$ & $\mathbf{1.2832}$ & $\mathbf{0.3049}$ \\
                    & $5$ ($70\%$)       & $\mathbf{0.0139}$ & $0.7405$          & $5.0714$          & $0.4717$          \\
        % & $6$ ($83.3\%$) & $0.0762$ & $1.0359$ & $204.1844$ & $0.4611$ \\
        % & $7$ ($96.7\%$) & $-0.0187$ & $0.5039$ & $1.6318$ & $0.3620$ \\ 
        \hline
        \multirow{3}{*}{mix}
        % & $1$ ($8.33\%$) & $-0.0563$ & $0.5211$ & $1.3403$ & $0.3813$ \\
        % & $2$ ($15.00\%$) & $-0.0040$ & $0.3095$ & $0.8648$ & $0.2269$ \\
        % & $3$ ($21.67\%$) & $0.0003$ & $0.2273$ & $0.6676$ & $0.1688$ \\
                    & $4$ ($28.33\%$)    & $-0.0033$         & $0.1814$          & $0.5627$          & $0.1353$          \\
        % & $5$ ($35.00\%$) & $-0.0014$ & $0.1490$ & $0.5054$ & $0.1111$ \\
        % & $6$ ($41.67\%$) & $0.0072$ & $0.1219$ & $0.4597$ & $0.0908$ \\
        % & $7$ ($48.33\%$) & $-0.0005$ & $0.0918$ & $0.4051$ & $0.0685$ \\
        % & $8$ ($55.00\%$) & $-0.0009$ & $0.0633$ & $0.3594$ & $0.0470$ \\
                    & $9$ ($61.67\%$)    & $\mathbf{0.0001}$ & $0.0319$          & $0.3143$          & $0.0237$          \\
        % & $10$ ($68.33\%$) & $-0.0004$ & $0.0128$ & $0.2573$ & $0.0093$ \\
        % & $11$ ($75.00\%$) & $-0.0006$ & $0.0085$ & $0.2043$ & $0.0061$ \\
        % & $12$ ($81.67\%$) & $-0.0002$ & $0.0027$ & $0.1339$ & $0.0019$ \\
                    & $13$ ($88.33\%$)   & $-0.0003$         & $\mathbf{0.0026}$ & $\mathbf{0.0589}$ & $\mathbf{0.0017}$ \\
        \bottomrule
    \end{tabular}
\end{table*}

We trained the GNNAEs to reconstruct the particle momenta in lab Cartesian coordinates, $(p_x, p_y, p_z)$, for a direct comparison with the LGAEs.
The LGAE was trained for about 200 epochs, whereas the GNNAE needed more than 1000 epochs to converge to an acceptable reconstruction performance.
Figures~\ref{fig:recons-hist-gnnae_cartesian} and \ref{fig:recons-jet_images-gnnae_cartesian} show the distribution and jet-image reconstruction by a GNNAE model with particle-level compression that was trained to reconstruct the particle momenta in the lab Cartesian coordinates.
The reconstructions of jet mass and jet images are worse than the LGAE at a similar level of compression, which is shown in \cref{fig:recons-jet-imgs-mix,fig:recons-hist}.

Figure~\ref{fig:recons-corr-gnnae_cartesian} shows the correlation plots between the target and reconstructed particle momenta by the two models. Qualitatively, the LGAE's reconstruction shows a stronger correlation with the target than the GNNAE's. Quantitatively, in terms of the correlation coefficient $r$, the reconstructions by the LGAE are better than the GNNAE at a similar level of compression. Note that although the $r$ values for the $\phi$ reconstruction have a similar order of magnitude, the negative value in the one by GNNAE indicates that a positive target $\phi^\mathrm{rel}$ is likely to be reconstructed as a negative value by the GNNAE, indicating a poor reconstruction.

% We also used two general correlation coefficients--Spearman's $\rho$, which measures the monotonicity of correlation, and Kendall's $\tau$ coefficient, which measures ordinal association--to measure the correlation. The higher $\rho$ in the LGAE's reconstruction indicates that increasing reconstructed features implies increasing target features with more confidence. The higher $\tau$ in the LGAE's reconstruction indicates that highly-ranked values of reconstructed features imply a higher rank in the corresponding target feature ordering. Both scores describe the stronger associations between the reconstructed and target feature in LGAE's reconstruction than in GNNAE's. 

\begin{figure*}[ht]
    \centering
    \includegraphics[scale=0.45]{figures/reconstructions/gnnae-cartesian/gnnae_cartesian-particle.pdf}
    \includegraphics[scale=0.45]{figures/reconstructions/gnnae-cartesian/gnnae_cartesian-jet.pdf}
    \caption{Particle momenta $(p_\mathrm{T}^\mathrm{rel}, \eta^\mathrm{rel}, \phi^\mathrm{rel})$ (top) and jet feature $(M, P_\mathrm{T}, \eta, \phi)$ (bottom) reconstructions by the GNNAE model with particle-level aggregation and the latent dimension of $\dim(L) = 2 \times 30$ when the model is trained to reconstruct $(p_x, p_y, p_z)$ at epoch 1001.}
    \label{fig:recons-hist-gnnae_cartesian}
\end{figure*}

\begin{figure*}[ht]
    \centering
    \includegraphics[height=0.8\paperheight]{figures/reconstructions/gnnae-cartesian/gnnae_cartesian-jet_images.pdf}
    \caption{Jet image reconstructions by the GNNAE model with particle-level aggregation and the latent dimension of $\dim(L) = 2 \times 30$ when the model is trained to reconstruct $(p_x, p_y, p_z)$ at epoch 1001.}
    \label{fig:recons-jet_images-gnnae_cartesian}
\end{figure*}

\begin{figure*}[ht]
    \centering
    \includegraphics[width=\linewidth]{figures/reconstructions/gnnae-cartesian/gnnae-recons-corr.pdf}
    \includegraphics[width=\linewidth]{figures/reconstructions/gnnae-cartesian/lgae-recons-corr.pdf}
    \caption{Correlations between the target particle momenta $(p_\mathrm{T}^\mathrm{rel}, \eta^\mathrm{rel}, \phi^\mathrm{rel})$ and reconstructed particle momenta by the GNNAE model with particle-level aggregation and the latent dimension of $\dim(L) = 2 \times 30$ (top) and by the LGAE model with mix aggregation and the $\tau_{(1/2, 1/2)} = 9$ latent 4-vectors (bottom).}
    \label{fig:recons-corr-gnnae_cartesian}
\end{figure*}

\subsubsection*{Learning Identity Mapping}
To see if the LGAEs and GNNAEs can reconstruct the jet when the latent space is large enough, we show reconstructions of particle-feature distribution and jet images by the LGAE at $88.3\%$ compression and the GNNAE with the latent dimension with no compression in \cref{fig:recons-hist-best,fig:recons-jet-imgs-best}, respectively.
In addition, \cref{fig:recons-hist-best} also shows the jet feature reconstruction by the LGAE model.

We see that the LGAE performs jet-image reconstruction decently and the particle-feature and jet-feature distribution almost perfectly, whereas the GNNAE still cannot have a very accurate reconstruction of the particle-feature distribution---especially the $p_\mathrm{T}^\mathrm{rel}$-distribution---and average jet image.
Therefore, we conclude that the LGAE can approximate the identity mapping better than the GNNAE when the latent space dimension is close enough to the dimension of physical data.

\begin{figure*}[ht]
    \centering
    \includegraphics[width=0.8\linewidth]{figures/reconstructions/best-models/polarrel-mix.pdf}
    \includegraphics[width=0.8\linewidth]{figures/reconstructions/best-models/jet.pdf}
    \caption{
        \textbf{Top}: Particle momenta $(p_\mathrm{T}^\mathrm{rel}, \eta^\mathrm{rel}, \phi^\mathrm{rel})$ reconstruction by the best-performance LGAE and GNNAE models.
        \textbf{Bottom}: Jet feature $(M, p_\mathrm{T}, \eta)$ reconstruction by the best-performance LGAE model.
        The best LGAE model is chosen to be that with mix aggregation and $\tau_{(1/2,1/2)}=13$ latent 4-vectors (resulting in $88.3\%$ compression).
        The best GNAE model is chosen to be that with particle-level aggregation and the latent dimension of $\dim(L) = 3 \times 30$ (resulting in no compression).
    }
    \label{fig:recons-hist-best}
\end{figure*}

\clearpage
\begin{figure*}[ht]
    \centering
    \includegraphics[height=0.75\paperheight]{figures/reconstructions/best-models/jet_images-mix.pdf}
    \caption{Jet image reconstructions by the best-performance LGAE (middle column) and GNNAE (right column) models.
        The best LGAE model is chosen to be that with mix aggregation and $\tau_{(1/2,1/2)}=13$ aggregation (resulting in $88.3\%$ compression).
        The best GNAE model is chosen to be that with particle-level aggregation and the latent dimension of $\dim(L) = 3 \times 30$ (resulting in no compression).
    }
    \label{fig:recons-jet-imgs-best}
\end{figure*}
